# Supplementary material for: Forget-Me-Not: Learning to Forget in Text-to-Image Diffusion Models
Source: arXiv:2303.17591 source file (2023-03-30)
Supplement: Supplementary file 1 [file appendix.tex]

\appendix
\section{ForgetBench}
\label{app:forgetbench}

\section{}
